# Supplementary material for: Two-step growth mechanism of the solid electrolyte interphase in argyrodyte/Li-metal contacts
Source: arXiv:2402.04095 source file (2024-02-06)
Supplement: Supplementary file 1 [file SI.pdf]

# Supporting information for "Two-step growth mechanism of the Solid Electrolyte Interphase in argyrodyte/Li-metal contacts"

Gracie Chaney,[1] Andrey Golov,[2] Ambroise van Roekeghem,[1] Javier Carrasco,[2,3] and Natalio Mingo[1]

[1)] *Université Grenoble Alpes, CEA, LITEN, 17 rue des Martyrs, 38054 Grenoble, France*

[2)] *Centre for Cooperative Research on Alternative Energies (CIC energiGUNE), Basque Research and Technology Alliance (BRTA), Alava Technology Park, Albert Einstein 48, 01510 Vitoria-Gasteiz, Spain*

[3)] *Ikerbasque, Basque Foundation for Science, Plaza Euskadi 5, 48009 Bilbao, Spain*

This supporting information includes details on the MD and machine learning computational methods, results for smaller size systems, details about active learning and cross-validation, and arguments supporting the percolation origin of the reaction slowdown phenomenon.

## S1. COMPUTATIONAL METHODS

An overview of the training set generation, energy and force calculation, and MLIP training is given below.

### A. Molecular Dynamics simulations

The dynamical evolution of the system is followed for 10 ns in an NPT ensemble with a Nosé-Hoover thermo- and barostat. For each system, we investigated three temperatures (300 K, 350 K, and 400 K), two internal pressures (1 bar and 1 kbar), and two random seeds for initializing the velocities. We used a 1 femtosecond (fs) timestep for all systems, except for the model II interface system at 400 K, 1 bar, seed 2, which required 0.5 fs timesteps to avoid instability.

### B. Training Set

In general, our training set consists of structural descriptors as inputs and DFT data (energies and forces) as target values. We created our initial 2732-configuration training set, using some of the AIMD results of Golov and Carrasco's 2021 paper.[1] Using active learning, described in III-C, we are able to grow and refine our training set.

### C. MLIP-2

MLIP-2 defines the local interatomic potential of an atom as a linear expansion of basis functions that are polynomial and consist of moments of inertia. These moments of inertia are the structural descriptors, consisting of radial and angular information about the local environment. A cutoff radius must be set by the user at the beginning of training to ensure smooth behavior of the radial basis functions. We chose a cutoff of 5.0 Å. It is also necessary for the user to choose the *level* of moments of the starting potential. The general rule is that a higher *level* increases the accuracy but extends the time of MLIP training. We tested a few *levels* before choosing a value of 8. We note that a newer version of MLIP has recently been released, but we did not use it in these calculations.[2]

## D. Active Learning

Traditionally, ML models have relied on large training sets whose qualities can determine the accuracy and predictive usefulness of the model itself. Thus, a pre-step to training is often examining and refining the training data. Such a process can be tedious, time-consuming, and may even bias the data if the refining is done manually. An alternative is active learning, which is an automated process that expands the data set by selecting configurations that lead to extrapolation. Fig 3 of Novikov's 2020 paper[3] illustrates the basic active learning process including (B) finding new structures in the training set and (D) calculating the energies and forces for the new structures. MLIP-2 determines which structures to add to the training set with the D-optimality criterion, based off of the extrapolation-grade limits, set by the user. The extrapolation-grade limits determine the ranges in which the active learning algorithm may select a non-redundant structure to add to the training-set. We gradually decrease the upper extrapolation grade from 5.5 to 2.5, while keeping the lower extrapolation grade at 1.5.

## E. Model Accuracy

We determine when to end active learning by examining the training-set size over time. As seen in Fig. S2, the active learning algorithm stops selecting new configurations after 40 iterations. That means the configuration space has already been explored enough to achieve a reliable accuracy.

We use k-fold cross-validation to determine the accuracy of our final model on both training and test sets. Specifically, we calculate the root-mean squared absolute difference errors on 10 k-fold samples. The mean energy/atom errors are 18.36 meV/atom and 20.89 meV/atom for the training and test sets respectively.

## F. Tracking total amount of reduction

We can track the amount of reduced electrolyte by analyzing the phosphorus coordination numbers. Throughout the reduction reaction, P atoms change their oxidation state from +5 to -3:

$Li_6^+P^{5+}S_5^{2-}Cl^- + 8Li^0 \rightarrow 5Li_2^+S^{2-} + Li^+Cl^- + Li_3^+P^{3-}$.

The electrolyte reduction can be viewed as a stepwise breaking of P-S bonds:

$(P^{5+}S_4^{2-})^{3-}$ + $2e^-$ $\rightarrow (P^{3+}S_3^{2-})^{3-}$ + $S^{2-}$

$(P^{3+}S_3^{2-})^{3-}$ + $2e^-$ $\rightarrow$ $(P^{+}S_2^{2-})^{3-}$ + $S^{2-}$

$(P^{+}S_2^{2-})^{3-}$ + $2e^-$ $\rightarrow$ $(P^{-}S^{2-})^{3-}$ + $S^{2-}$

$(P^{-}S^{2-})^{3-}$ + $2e^-$ $\rightarrow$ $P^{3-}$ + $S^{2-}$

According to the equation, the complete reduction of one formula unit of the electrolyte requires 8 electrons. Consequently, for Z formula units, 8 Z electrons are required. At any step of molecular dynamics, the number of electrons transferred from metal Li to the electrolyte can be found from the number (N) of partially and completely reduced thiophosphate groups. Thus, the percentage of reduced argyrodite ($\alpha$) can be calculated using the following formula: $\alpha$ =(8N(P)+6N(PS)+4N($PS_2$)+2N($PS_3$))/8Z

The P-S coordination numbers were calculated based on a distance criterion of 3Å.

## G. Tracking crystallization

To track the crystallization of the reaction products at the Li/LPSC interface we employed a previously developed approach based on graph algorithms and the concept of natural tiling.[4] Natural tiling is the division of a structure into minimal intra-framework cages (tiles), forming periodic space-filling tessellation. Tiles can be represented as structure-building units and used for the description of crystal growth.[4] According to AIMD simulations, the product of the reaction argyrodite with Li is $5Li_2S{\cdot}Li_3P{\cdot}LiCl$ solid solution, which belongs to the antifluorite structure type.[4] The natural tiling of this structure is a rhombic dodecahedral honeycomb. Thus, the crystalline region can be identified as a set of adjacent rhombic dodecahedra. This is accomplished using a subgraph search algorithm. The graph of the crystal structure is defined by Li-X (where, X=S, Cl, and P) neighboring pairs of atoms, determined based on Voronoi decomposition.[5] The subgraph search employs the Glasgow subgraph solver.[6]

We define the SEI crystallinity as a percentage, given by $100 \times N/(21Z)$, where $N$ is the number of atoms within the crystalline region, Z is the number of formula units of electrolyte within the structure, and 21 the number of atoms within the reaction product $5Li_2S{\cdot}Li_3P{\cdot}LiCl$ that forms from the reaction of one formula unit of electrolyte with 8 atoms of Li.

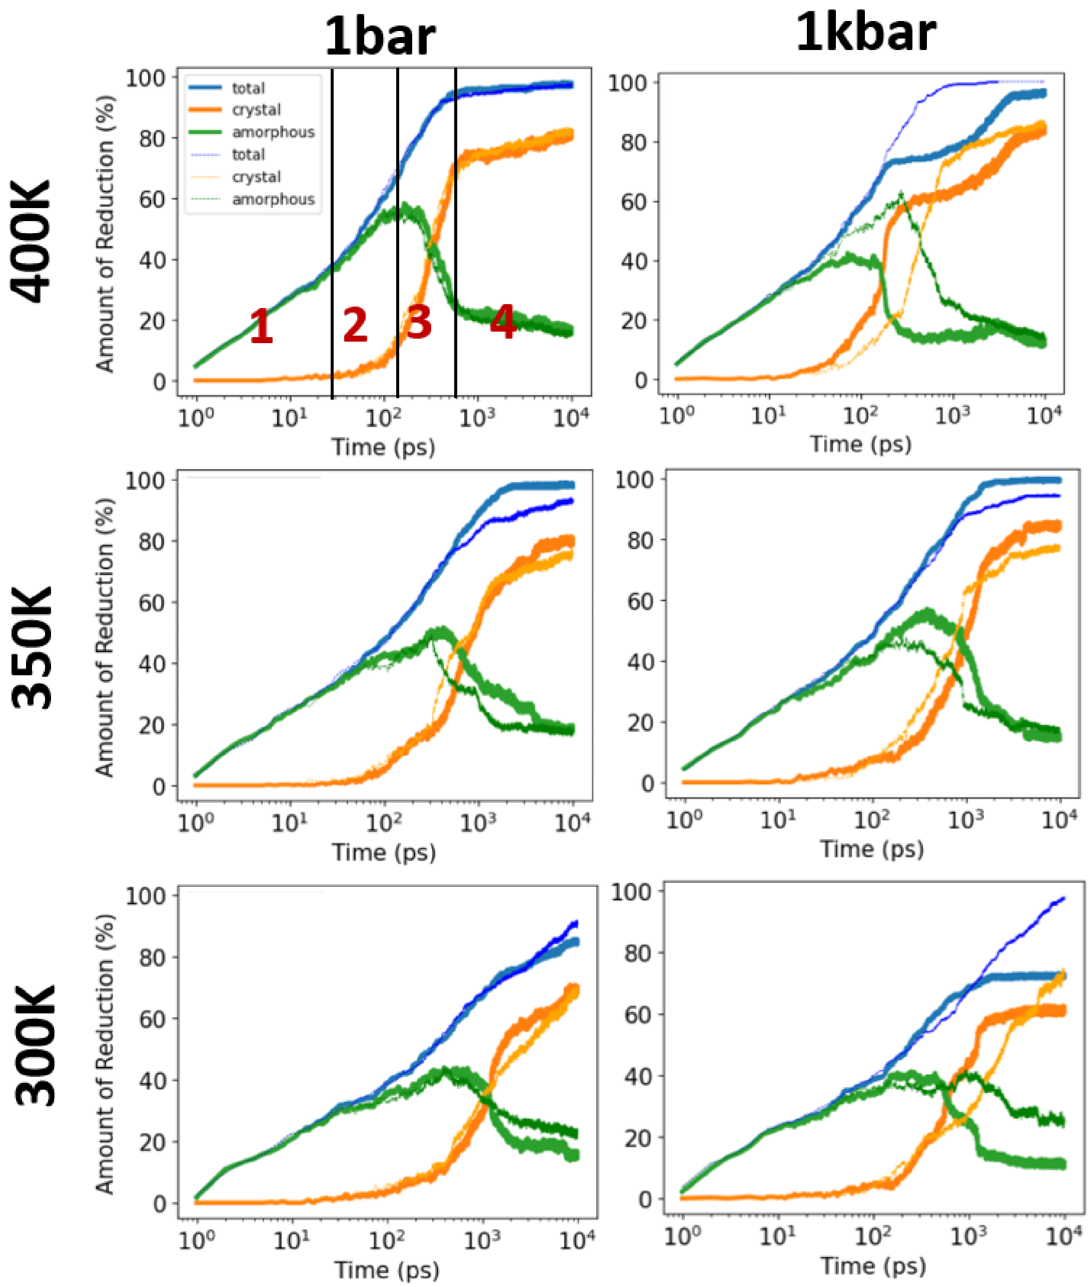


FIG. S1: Amount of reduction vs time for crystalline, amorphous, and overall reduced regions of electrolyte. Shown for two MD seeds, distinguished by different line thicknesses. Calculations performed on model I interface of Li-anode/LPSC. The four time-regimes are illustrated in the top-left plot and described in the main paper.

## S2. PHASE EVOLUTION CURVES FOR THE MODEL I INTERFACE

The model I interface (7956-atoms) displays interesting behaviors that we did not observe in the simulations for the model II interface shown in the main text (Fig. S1). Besides the large influence of the velocity seed (discussed in the main text), this smaller system also shows a Li-diffusion bottleneck effect (a sudden slow down of the reaction) in some cases where a significant fraction of the original argyrodite has not yet been reduced. We provide an explanation for this phenomenon in section S4 below.

## S3. ACTIVE LEARNING AND CROSS VALIDATION ERRORS

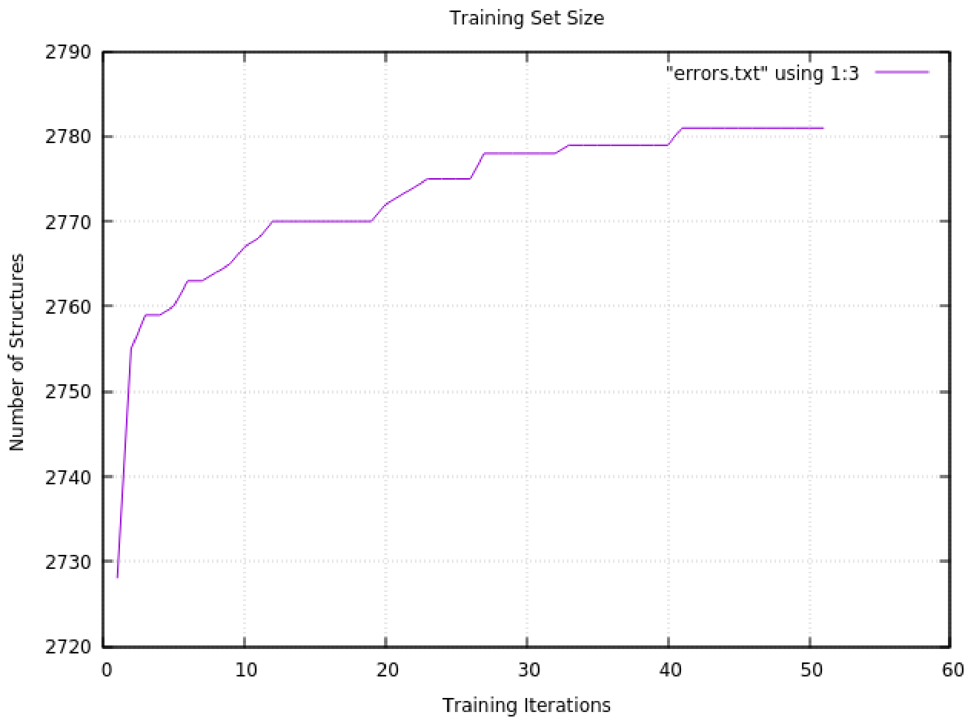


FIG. S2: Number of structures in training-set vs MLIP training iterations. Active learning stops selecting new structures after about 40 iterations. The initial training set comprised 2732 structures.

| Fold | Training Set Size | Test Set Size | Training Errors | Testing Errors |
|---|---|---|---|---|
| 1 | 2506 | 275 | 0.0184648 | 0.0160566 |
| 2 | 2503 | 278 | 0.0182038 | 0.0156830 |
| 3 | 2503 | 278 | 0.0185344 | 0.0174717 |
| 4 | 2503 | 278 | 0.0180033 | 0.0328334 |
| 5 | 2503 | 278 | 0.0189997 | 0.0210023 |
| 6 | 2506 | 275 | 0.0186082 | 0.0131903 |
| 7 | 2503 | 278 | 0.0187420 | 0.0174633 |
| 8 | 2503 | 278 | 0.0180340 | 0.0178399 |
| 9 | 2503 | 278 | 0.0182212 | 0.0332638 |
| 10 | 2496 | 285 | 0.0178247 | 0.0240829 |

TABLE S1: RMS absolute energy difference (eV/atom) for training and test sets in a 10-fold cross-validation.

## S4. DIFFUSION BOTTLENECK

The 1 kbar / 400 K / seed 1 case in figure S1 shows that the total reduction suddenly stalls at about 200 ps, and then picks up at a much slower rate. This seems to be due to a closing of the amorphous channels that connect the electrode and unreacted electrolyte. The resulting continuous layer of crystalline $Li_2(SPCl)$ solid solution has a much lower ionic conductivity than the amorphous phase, thus impeding Li inflow and clogging the reaction. This can be seen in the figure below, which shows the atoms corresponding to the crystalline phase at different time steps.

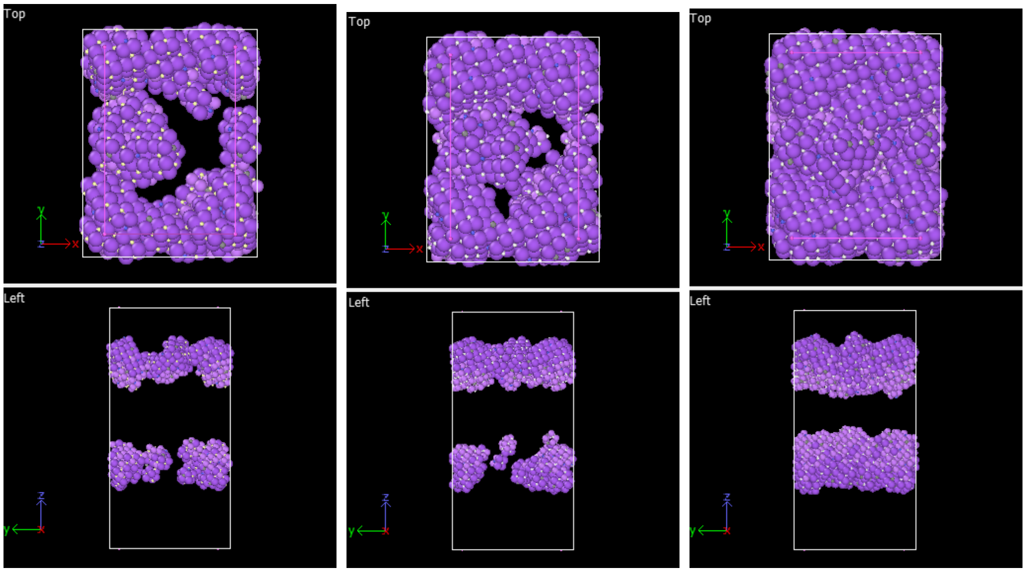


FIG. S3: Top and side views of the atoms belonging to the crystalline region in the 400 K, 1 kbar, seed 1, 3x3 system, at 100 ps, 150 ps, and 200 ps respectively. A continuous layer has formed at 200 ps, preventing Li inflow, and stalling the reaction, despite the fact that there is still a considerable amount of unreacted argyrodite in the system.

## S5. ATOMIC CONFIGURATIONS AT 10 NS

For the sake of clarity, Fig. 3 of the main text only shows snapshots of the model II interface up to 1 ns, time at which the electrolyte is not yet fully reduced. Here we show the same systems after 10 ns, which display a fully reduced polycrystalline electrolyte. As section S4 above shows for the model I simulations, it is possible to find systems where the reaction stalls before all the electrolyte is reduced, due to lack of percolation through the continuous crystalline layer. However, all our simulations for model II displayed complete reduction.

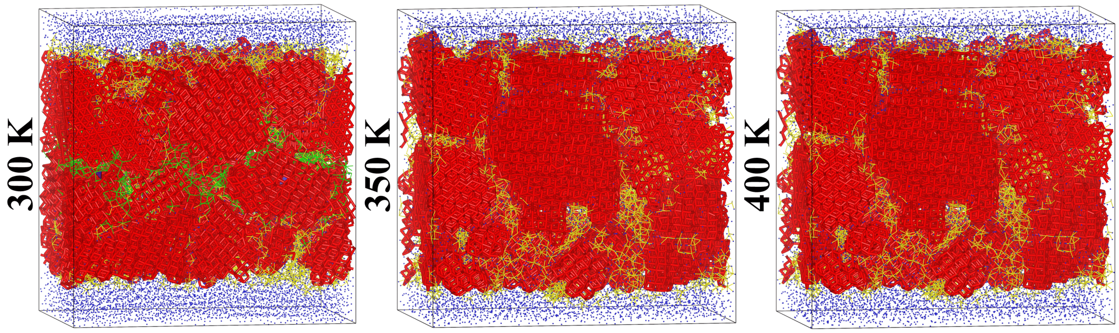


FIG. S4: Atomic configurations at 10 ns (complement to Fig. 3). Red: crystalline regions. Yellow: amorphous reduced regions. Blue dots: Li-metal. Purple polyhedra and green lines correspond to thiophosphate groups and Li- Cl, Li-S bonds, respectively, in the original argyrodite structure. The snapshots correspond to the model II interface for various temperatures at a pressure of 1 bar (seed no. 1 for the initial velocities.)

## BIBLIOGRAPHY

[1]A. Golov and J. Carrasco, "Molecular-level insight into the interfacial reactivity and ionic conductivity of a li-argyrodite $Li_6PS_5Cl$ solid electrolyte at bare and coated li-metal anodes," ACS Applied Materials  Interfaces **13**, 43734–43745 (2021).

[2]E. Podryabinkin, K. Garifullin, A. Shapeev, and I. Novikov, "MLIP-3: Active learning on atomic environments with Moment Tensor Potentials," (2023).

[3]I. S. Novikov, K. Gubaev, E. V. Podryabinkin, and A. V. Shapeev, "The mlip package: moment tensor potentials with mpi and active learning," Machine Learning: Science and Technology **2**, 025002 (2020).

[4]A. Golov and J. Carrasco, "Unveiling Solid Electrolyte Interphase Formation at the Molecular Level: Computational Insights into Bare Li-Metal Anode and $Li_6PS_{5-x}Se_xCl$ Argyrodite Solid Electrolyte," ACS Energy Letters **8**, 4129–4135 (2023).

[5]V. A. Blatov *, "Voronoi–dirichlet polyhedra in crystal chemistry: theory and applications," Crystallography Reviews **10**, 249–318 (2004).

[6]C. McCreesh, P. Prosser, and J. Trimble, "The Glasgow Subgraph Solver: Using Constraint Programming to Tackle Hard Subgraph Isomorphism Problem Variants," in *Graph Transformation*, Lecture Notes in Computer Science, edited by F. Gadducci and T. Kehrer (Springer International Publishing, Cham, 2020) pp. 316–324.
